# Supplementary material for: Optimal and Approximation Algorithms for Joint Routing and Scheduling in Millimeter-Wave Cellular Networks
Source: arXiv:2007.02621 source file (2020-07-06)
Supplement: Supplementary file 1 [file real-su-sm.tex]

\section{Algorithms for the REAL-SU-SM Model}
This section deals with the MTFS scheduling algorithms (optimal and approximation) assuming the single user spatial multiplexing model MAX-SU-SM (see Sec.~\ref{sec:su-sm}).

\subsection{Optimal FD-MTFS Scheduling Algorithm Assuming NI Model and REAL-SU-SM Model}
This section is actually an extension of the optimal FD-MTFS scheduling algorithm in Sec.~\ref{s:fd-sched-fair}.
The difference in the problem setting is that in  Sec.~\ref{s:fd-sched-fair} we assume the MAX-SU-SM model while in this section we assume REAL-SU-SM model.
In the following, we will list the modification to the algorithm for the REAL-SU-SM model.

Instead of optimizing on the expanded network $H$, we now optimize on the multi-arc network $F$. $F$ has the same vertex set as $D$, $V(F) = V(D)$.
Each arc $e \in E(D)$ is mapped into $d(e)$ number of parallel arcs $e_1 \dots e_{d(e)}$ where $d(e)$ is the maximum number of data streams for link $e$. The arcs have non-increasing capacities such that $c(e_k) = c_k(e)$. 

The FD-MTFS algorithm for the MAX-SU-SM model performs maximum weighted matching on the expanded network $H$ iteratively. 
Similarly, the FD-MTFS algorithm for REAL-SU-SM model performs {\em maximum weighted simple $b$-matching}~\cite{Korte12} on the multi-arc network $F$ iteratively.
\begin{mydef}{Maximum Weighted Simple $b$-matching.} Let $G$ be an undirected graph with numbers $b: V(G) \mapsto \mathbb{N}$ and weights $c: E(G) \mapsto \mathbb{R}$, then a {\em simple $b$-matching} in $G$ is a function $f: E(G) \mapsto \{0, 1\}$ and $\sum_{e \in \delta(v)} f(e) \le b(v)$ for all $v \in V(G)$ where $\delta(v)$ is the set of edges incident to $v$. A {\em maximum weighted simple $b$-matching} $f$ is a simple $b$-matching whose weight $\sum_{e \in E(G)} c(e) f(e)$ is maximum.
\end{mydef}

Analogously, the FD-MTFS problem for the REAL-SU-SM model can be mathematically formulated with the help of the {\em node-simple-$b$-matching matrix}.
\begin{mydef}{Node-$b$-matching Matrix.}
	Given a multi-arc network $F$, suppose the number of all possible simple $b$-matching in $F$ is $K$.
	Then the node-$b$-matching matrix $\mat{A} = [a_{i, j}]$ is a $|V(F)| \times K$ matrix. Each element $a_{i, j}$ is equal to the sum capacity of all arcs in the $j$-th simple $b$-matching that enter the $i$-th vertex minus the sum capacity of all arcs in the simple $j$-th $b$-matching that leave the $i$-th vertex.
\end{mydef} 

\begin{figure}[!hbpt]
	\begin{minipage}{0.3\textwidth}
		\begin{figure}[H]
			\includegraphics[width=8cm]{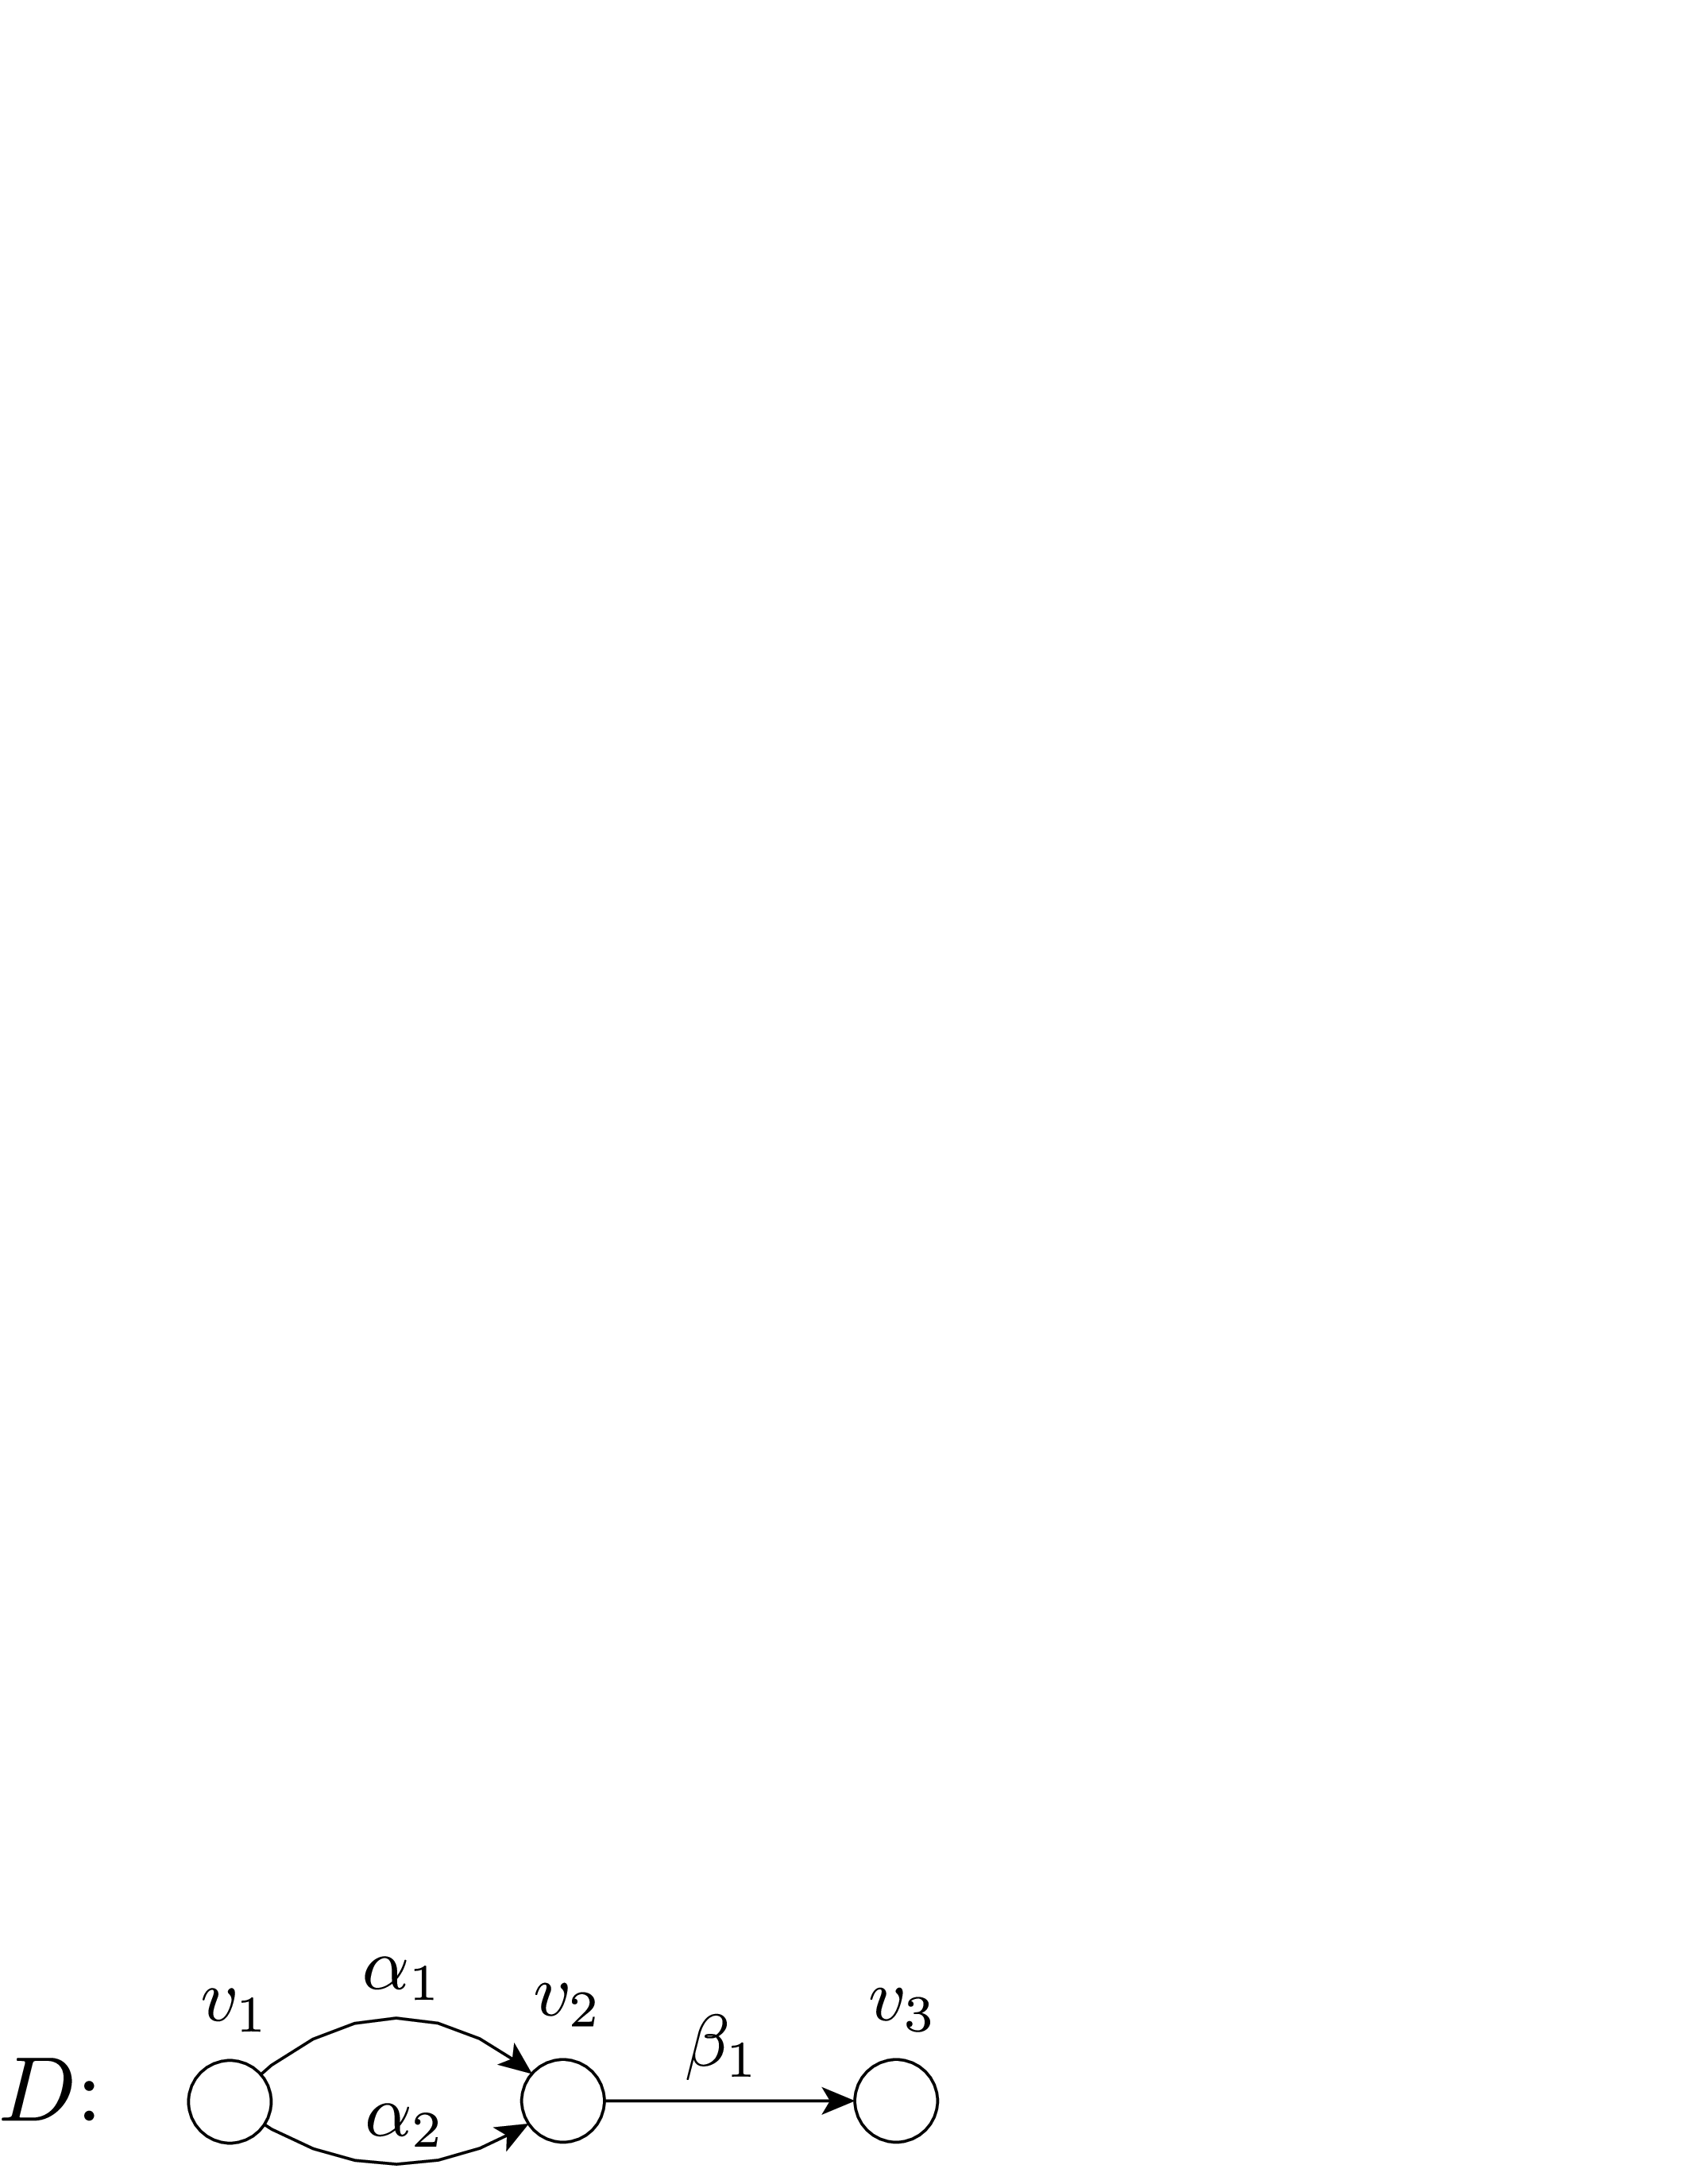}	
		\end{figure}
	\end{minipage} \\ \\ \\ 
	$\mat{A:}$
	\begin{minipage}{0.7\textwidth} \footnotesize
		$\begin{blockarray}{ccccccccccccccccc}
		& \alpha_1  & \alpha_2  & \beta_1  & \alpha_1,\alpha_2  & \alpha_1, \beta_1  & \alpha_2, \beta_1 \\
		\begin{block}{c[cccccccccccccccc]}
		v_0  & -8 & -6 & 0   & -14 & -8 & -6  \\
		v_1  & 8  & 6  & -3  & 14  & 5  & 3 \\
		v_2  & 0  & 0  & 3   & 0   & 3  & 3  \\
		\end{block}
		\end{blockarray}$
	\end{minipage}
	\caption{Node-$b$-matching matrix $\mat{A}$. $v_0, v_1$ and $v_2$ are the nodes in backhaul network, each with 2 RF chains.
		The maximum number of data streams of each link is $d(\alpha) = 2, d(\beta) = 1$.
		 The arc capacities in the multi-arc network $F$ are: $c(\alpha_1) = 8$, $c(\alpha_2) = 6$, $c(\beta_1) = 3$.}
	\label{fig:node-b-matching}
\end{figure}

Fig.~\ref{fig:node-b-matching} gives an example of the node-$b$-matching matrix. Correspondingly, we define $\mat{A}^M$ as the submatrix of $\mat{A}$ related to the relay BSs in $F$. The set of arcs scheduled in each timeslot must be a simple $b$-matching in $F$. We define $\vect{c}$ as {\em capacity vector} whose element $c_j$ is the cumulative capacity of all macro-BS-to-relay-BS data streams in the $j$-th simple $b$-matching $M_j$, i.e.,
$c_j = \sum_{\{e | e \in M_j, \text{tail}(e) \in B(F) \}} c(e)$ where $B(F)$ are the vertex set of macro-BSs in $F$.
Consequently, the linear program formulation for the FD-MTFS problem for the REAL-SU-SM model is exactly the same as \eqref{eq:mtf-theta} and \eqref{eq:mtf}.
It can be solved in polynomial time by Alg.~\ref{alg:mtf-theta} and \ref{alg:mtf} with slight modification.
Line \ref{alg:mtf-a1} of Alg.~\ref{alg:mtf-theta} is replaced by:

\small
Set weight $w(e_m)$ to each arc $e_m = (v_i, v_j)_m \in E(F)$ where
\begin{equation*}
w(e_m) \eqdef
\begin{cases}
c(e_m) (p_j - p_i) & \text{if }v_i \in M(D)
\\
c(e_m) p_j         & \text{otherwise}.
\end{cases} 
\end{equation*}
Do max weighted simple $b$-matching on $F$ and let the max weight be $z$.  Compute $\eta_1 = -z - p_{\card{M(D)}+1}$
\normalsize

Line \ref{alg:mtf-b1} of Alg.~\ref{alg:mtf} is replaced by:

\small
Set weight $w(e_m)$ to each arc $e_m = (v_i, v_j)_m \in E(F)$ where
\begin{equation*}
w(e_m) \eqdef 
\begin{cases}
c(e_m) (p_j - p_i) & \text{if }v_i \in M(D) \\
c(e_m) (p_j + 1)   & \text{otherwise}.
\end{cases}
\end{equation*}
Do max weighted simple $b$-matching on $F$ and let the max weight be $z$. Compute $\eta_1 = -z - p_{\card{M(D)}+1}$
\normalsize

The initial basic solution to \eqref{eq:mtf-theta} is constructed by replacing $H'$ with $F'$ which is a subgraph of $F$ such that $E(F') = \{e_1 | e \in E(D)\}$. Analogously, the FD-MTFS problem for the REAL-SU-SM model can be solved in polynomial time.
\begin{thm}
	\label{thm:Fd-MTFS-REAL-poly}
	The FD-MTFS problem for the REAL-SU-SM model can be solved in polynomial time with the ellipsoid algorithm.
\end{thm}
